# Supplementary material for: Generalized Total Internal Reflection at Dynamic Interfaces
Source: arXiv:2208.07759 ancillary file (2022-08-17)
Supplement: Supplementary file 1 [file Supplementary_Material_for_Generalized_Total_Internal_Reflection_at_Dynamic_Interfaces.pdf]

# Supplementary Material for "Generalized Total Internal Reflection at Dynamic Interfaces"

Zhiyu Li,[1,2,*] Xikui Ma,[1] Amir Bahrami,[2] Zoé-Lise Deck-Léger,[3] and Christophe Caloz[2]

[1] *State Key Laboratory of Electrical Insulation and Power Equipment, School of Electrical Engineering, Xi'an Jiaotong University, Xi'an, Shaanxi, China*

[2] *Department of Electrical Engineering, KU Leuven, Leuven, Belgium*

[3] *Department of Electrical Engineering, Polytechnique Montréal, Montréal, Quebec, Canada*

(Dated: August 17, 2022)

## CONTENTS

I. Explanation of the Inexistence of the TIR phenomenon in the Superluminal-Modulation Domino-Chain System 2

A. Derivation of the Scattered Angle Formulas 2
B. Impossibility to Satisfy the TIR Criterion 2

II. Moving Matter Bianisotropy 3

III. Incidence and Reflection Angles versus Transmission Phase Angle 4
A. Derivation of $\theta_{\mathrm{i}}(\mathbf{k}_{\mathrm{t}})$ 4
B. Derivation of $\theta_{\mathrm{r}}(\mathbf{k}_{\mathrm{t}})$ 5

IV. Derivation of the Critical Angle Equations in Table I 6
A. Conveyor-Belt System [Fig. 1(b), Eqs. (2)] 6
1. Frame-Hopping Method 6
2. Catch-Up Method 7
B. Domino-Chain System [Fig. 1(c), Eqs. (c)] 7
1. Frame-Hopping Method 7
2. Catch-Up Method 8
C. Moving-Truck System [Fig. 1(d), Eqs. (4)] 8
1. Frame-Hopping Method 8
2. Catch-Up Method 9

V. Derivation for the Most General Moving Interface – Moving matter System ($v \neq v_{\mathrm{m}}$) 11
A. Catch-Up Criterion 11
B. Critical Transmission Group and Phase Angles 11
C. Critical Incidence and Reflection Angles 11
1. Stationary Interface – Moving Matter System: the Conveyor-Belt System 12
2. Moving Interface – Stationary Matter System: the Domino-Chain System 12
3. Moving Interface – Moving Matter System ($v = v_{\mathrm{m}}$): Moving-Truck System 12

VI. Catch-Up Graphs for the Three Systems in Fig. 1 (a)-(c) 13

VII. Generalized Snell's Law and Momentum diagram 15
A. Snell's Law for Transmission 15
1. General Case 15
2. Particular Cases 15
B. Snell's Law for Reflection 16
1. General Case 16
2. Particular Cases 16
C. Momentum Diagram with Reflection 16

VIII. Full-Wave Simulation Results 18

References 18

# I. EXPLANATION OF THE INEXISTENCE OF THE TIR PHENOMENON IN THE SUPERLUMINAL-MODULATION DOMINO-CHAIN SYSTEM

## A. Derivation of the Scattered Angle Formulas

For superluminal modulation systems, where the modulation (interface) velocity is larger than the maximum velocity of light in the two media ($v > c/n_{\min}$), we choose the $K'$ frame as being a simultaneity frame, whose velocity is $v_{\mathrm{f}} = c^2/v$ [1]. In the $K'$ frame, the moving interface is purely temporal and we have therefore the temporal boundary condition

$$k'_{z_{\mathrm{i}}} = k'_{z_{\mathrm{r}}} = k'_{z_{\mathrm{t}}} \tag{S1a}$$

and

$$k'_{x_{\mathrm{i}}} = k'_{x_{\mathrm{r}}} = k'_{x_{\mathrm{t}}}. \tag{S1b}$$

Applying the spectrum Lorentz transformation, $k'_z = \gamma(k_z \mp \beta\omega'/c)$ and $k'_x = k_x$, where $\beta = v_{\mathrm{f}}/c = c/v$, and using the dispersion relations of the two isotropic media, $k = \omega n/c$, we find the boundary condition in the laboratory frame, the $K$ frame, as

$$k_{\mathrm{i}}(\cos\theta_{\mathrm{i}} - \beta/n_1) = k_{\mathrm{r}}(\cos\theta_{\mathrm{r}} + \beta/n_2) = k_{\mathrm{t}}(\cos\theta_{\mathrm{t}} - \beta/n_2) \tag{S2a}$$

and

$$k_{x_{\mathrm{i}}} = k_{x_{\mathrm{r}}} = k_{x_{\mathrm{t}}}. \tag{S2b}$$

Then, dividing Eq. (S2b) by Eq. (S2a), we obtain the superluminal Snell's law

$$\frac{\sin\theta_{\mathrm{i}}}{\cos\theta_{\mathrm{i}} - \beta/n_1} = \frac{\sin\theta_{\mathrm{r}}}{\cos\theta_{\mathrm{r}} + \beta/n_2} = \frac{\sin\theta_{\mathrm{t}}}{\cos\theta_{\mathrm{t}} - \beta/n_2}. \tag{S3}$$

Solving Eq. (S3) for the reflection and transmission angles, we finally get

$$\cos\theta_{\mathrm{r}} = \frac{\beta n_1^2(1-\cos^2\theta_{\mathrm{i}}) + (\beta - n_1\cos\theta_{\mathrm{i}})\sqrt{n_2^2(\beta^2 - 2\beta n_1\cos\theta_i + n_1^2) - n_1^2\beta^2(1-\cos^2\theta_{\mathrm{i}}))}}{n_2(\beta^2 - 2\beta n_1\cos\theta_{\mathrm{i}} + n_1^2)} \tag{S4a}$$

and

$$\cos\theta_{\mathrm{t}} = \frac{-\beta n_1^2(1-\cos^2\theta_{\mathrm{i}}) + (\beta - n_1\cos\theta_{\mathrm{i}})\sqrt{n_2^2(\beta^2 - 2\beta n_1\cos\theta_{\mathrm{i}} + n_1^2) - n_1^2\beta^2(1-\cos^2\theta_{\mathrm{i}}))}}{n_2(\beta^2 - 2\beta n_1\cos\theta_{\mathrm{i}} + n_1^2)}. \tag{S4b}$$

## B. Impossibility to Satisfy the TIR Criterion

According to the generalized TIR criterion, the TIR phenomenon occurs when the transmitted wave becomes evanescent, which, under the phase-matching boundary condition (continuity of $k_x$), occurs when $k_{z_{\mathrm{t}}}$ becomes complex. If $k_{z_{\mathrm{t}}}$ is complex in the $K$ frame, then $k'_{z_{\mathrm{t}}}$ is also complex in the $K'$ frame. According to the purely temporal boundary condition, $\Delta k'_z = 0$, the reflected wave must then also be evanescent, so that TIR cannot occur.

This can be mathematically shown as follows. According to Eqs. (S4), when the transmitted wave is evanescent, the radicand in the numerator of Eq. (S4b) is negative, and so will the radicand in the numerator of Eq. (S4a), which is equal to it. In this case, the transmitted wave and the reflected wave would be simultaneously evanescent, which would make TIR impossible.

## II. MOVING MATTER BIANISOTROPY

Consider an isotropic medium with static refractive index $n_2$ moving at relativistic velocity $v_{\rm m}$, as shown in Fig. 1(b) and (d). In the moving-matter frame, the $K'$ frame (different definition than in the body of the paper, where $K'$ represents the $K$-stationary interface in the conveyor-belt system), which moves at the same velocity $v_{\rm m}$ as the moving atoms and molecules in medium 2, the moving matter appears stationary. We have then the simple constitutive relations

$$\mathbf{D}' = \epsilon_2 \mathbf{E}' \quad \text{and} \quad \mathbf{B}' = \mu_2 \mathbf{H}', \tag{S5}$$

where $\epsilon_2$ and $\mu_2$ are the permittivity and permeability of the isotropic medium 2 at rest, respectively, and the rest refractive index is $n_2 = \sqrt{\epsilon_2 \mu_2}$.

Applying the Lorentz transformations of the field [1, 2] to Eq. (S5), we find the bianisotropic constitutive relations in the laboratory frame, the $K$ frame [3], as

$$\mathbf{D} = \overline{\overline{\epsilon}} \cdot \mathbf{E} + \overline{\overline{\xi}} \cdot \mathbf{H} \quad \text{and} \quad \mathbf{B} = \overline{\overline{\mu}} \cdot \mathbf{H} + \overline{\overline{\zeta}} \cdot \mathbf{E}, \tag{S6a}$$

where

$$\overline{\overline{\epsilon}} = \epsilon_2 \begin{bmatrix} \alpha_2 & 0 & 0 \\ 0 & \alpha_2 & 0 \\ 0 & 0 & 1 \end{bmatrix}, \quad \overline{\overline{\mu}} = \mu_2 \begin{bmatrix} \alpha_2 & 0 & 0 \\ 0 & \alpha_2 & 0 \\ 0 & 0 & 1 \end{bmatrix}, \quad \overline{\overline{\xi}} = \begin{bmatrix} 0 & \chi_2/c & 0 \\ -\chi_2/c & 0 & 0 \\ 0 & 0 & 0 \end{bmatrix} \quad \text{and} \quad \overline{\overline{\zeta}} = \overline{\overline{\xi}}^T, \tag{S6b}$$

with

$$\alpha_2 = \frac{1-\beta_{\rm m}^2}{1-\beta_{\rm m}^2 n_2^2} \quad \text{and} \quad \chi_2 = \beta_{\rm m} \frac{1-n_2^2}{1-\beta_{\rm m}^2 n_2^2}. \tag{S6c}$$

Substituting Eq. (S6) into Maxwell's equations and eliminating the field quantities $\mathbf{E}, \mathbf{H}, \mathbf{D}$ and $\mathbf{B}$, we obtain the dispersion relation [3, 4]

$$\left(k_z - \frac{\omega}{c}\chi_2\right)^2 + \alpha_2 k_x^2 = \left(\alpha_2 n_2 \frac{\omega}{c}\right)^2. \tag{S7}$$

The phase velocity is found by substituting $\omega = kc/n_2(\mathbf{k})$, $k_z = k\cos\theta^{\mathbf{k}}$ and $k_x = k\sin\theta^{\mathbf{k}}$ into Eq. (S7), which yields

$$\mathbf{v}_{\rm p} = \frac{c}{n_2(\mathbf{k})}\hat{\mathbf{k}} = \frac{c\left(\cos^2\theta^{\mathbf{k}} + \alpha_2 \sin^2\theta^{\mathbf{k}}\right)}{\chi_2 \cos\left(\theta^{\mathbf{k}}\right) \pm \sqrt{\chi_2^2 \cos^2\theta^{\mathbf{k}} - \left(\cos^2\theta^{\mathbf{k}} + \alpha_2 \sin^2\theta^{\mathbf{k}}\right)\left(\chi_2^2 - \alpha_2^2 n_2^2\right)}}\hat{\mathbf{k}}. \tag{S8}$$

The group velocity is found by taking the derivative of Eq. (S7) with respect to $k_z$ and $k_x$ separately, which yields

$$\mathbf{v}_{\rm g} = \nabla_{\mathbf{k}}\omega(\mathbf{k}) = \frac{\alpha_2 k_x \hat{\mathbf{x}} + \left(k_z - \omega\chi_2/c\right)\hat{\mathbf{z}}}{\omega\left(\alpha_2^2 n_2^2/c^2\right) + \chi_2/c\left(k_z - \omega\chi_2/c\right)}. \tag{S9}$$

Then, the group angle is calculated from Eq. (S9) as

$$\theta^{\mathbf{S}} = \arctan\left(\frac{v_{{\rm g}_x}}{v_{{\rm g}_z}}\right) = \arctan\left(\frac{\alpha_2 k_x}{k_z - \omega\chi_2/c}\right) = \arccos\left[\frac{k_z - \omega\chi_2/c}{\sqrt{\alpha_2^2 k_x^2 + \left(k_z - \omega\chi_2/c\right)^2}}\right], \tag{S10a}$$

while the phase angle is, by definition,

$$\theta^{\mathbf{k}} = \arctan\left(\frac{k_x}{k_z}\right) = \arccos\left(\frac{k_z}{\sqrt{k_z^2 + k_x^2}}\right). \tag{S10b}$$

## III. INCIDENCE AND REFLECTION ANGLES VERSUS TRANSMISSION PHASE ANGLE

Substituting $k=\omega n/c$, $k_x=k\sin\theta$ and $k_z=k\cos\theta$, with $n=n_1$ in medium 1 and $n=n_2(\mathbf{k}_\mathrm{t})$ in medium 2, into the boundary condition of the $K$ frame, we find the Snell's law relation (we use here $\theta_\mathrm{t}=\theta_\mathrm{t}^\mathbf{k}$ for simplicity)

$$\frac{\sin\theta_\mathrm{i}}{1/\beta n_1-\cos\theta_\mathrm{i}}=\frac{\sin\theta_\mathrm{r}}{-1/\beta n_1-\cos\theta_\mathrm{r}}=\frac{\sin\theta_\mathrm{t}}{1/\beta n_2(\mathbf{k}_\mathrm{t})-\cos\theta_\mathrm{t}}. \tag{S11}$$

While scattered angle formulas can take different forms, we use here the method in [5], which is based on Eq. (S11) and which is ideal to understand the influence of the interface motion.

### A. Derivation of $\theta_\mathrm{i}(\mathbf{k}_\mathrm{t})$

In Eq. (S11), we set

$$N=\frac{\sin\theta_\mathrm{i}}{1/\beta n_1-\cos\theta_\mathrm{i}}=\frac{\sin\theta_\mathrm{t}}{1/\beta n_2(\mathbf{k}_\mathrm{t})-\cos\theta_\mathrm{t}}, \tag{S12}$$

where the left equality leads to

$$\sin\theta_\mathrm{i}+N\cos\theta_\mathrm{i}=N/\beta n_1. \tag{S13}$$

Dividing both sides by $1/\sqrt{1+N^2}$ yields

$$\frac{\sin\theta_\mathrm{i}+N\cos\theta_\mathrm{i}}{\sqrt{1+N^2}}=\frac{N}{\beta n_1\sqrt{1+N^2}}, \tag{S14}$$

which may be rewritten as

$$\sin\theta_\mathrm{i}\cos\psi+\cos\theta_\mathrm{i}\sin\psi=\sin\left(\theta_\mathrm{i}+\psi\right)=\sin\phi, \tag{S15}$$

with the new angles $\psi$ and $\phi$, where $\cos\psi=1/\sqrt{1+N^2}$, $\sin\psi=N/\sqrt{1+N^2}$ and $\sin\phi=N/(\beta n_1\sqrt{1+N^2})$. Finally, inserting $N=\sin\theta_\mathrm{t}/[1/\beta n_2(\mathbf{k})-\cos\theta_\mathrm{t}]$ [Eq. (S12)] into $\sin\psi$ and $\sin\phi$, we get the relation between $\theta_\mathrm{i}$ and $\theta_\mathrm{t}$ as

$$\theta_\mathrm{i}=\phi-\psi, \tag{S16a}$$

with

$$\phi=\arcsin\left(\frac{N}{\beta n_1\sqrt{1+N^2}}\right)=\arcsin\left(\frac{n_2(\mathbf{k}_\mathrm{t})\sin\theta_\mathrm{t}}{n_1\sqrt{\beta^2 n_2(\mathbf{k}_\mathrm{t})^2-2\beta n_2(\mathbf{k}_\mathrm{t})\cos\theta_\mathrm{t}+1}}\right) \tag{S16b}$$

and

$$\psi=\arcsin\left(\frac{N}{\sqrt{1+N^2}}\right)=\arcsin\left(\frac{\beta n_2(\mathbf{k}_\mathrm{t})\sin\theta_\mathrm{t}}{\sqrt{\beta^2 n_2(\mathbf{k}_\mathrm{t})^2-2\beta n_2(\mathbf{k}_\mathrm{t})\cos\theta_\mathrm{t}+1}}\right). \tag{S16c}$$

Substituting the normalized dispersion relation of medium 2, $\overline{k}_\mathrm{t}=n_2(\mathbf{k}_\mathrm{t})$ (normalized to $\omega_\mathrm{t}/c$), $\overline{k}_{z_\mathrm{t}}=n_2(\mathbf{k}_\mathrm{t})\cos\theta_\mathrm{t}$ and $\overline{k}_{x_\mathrm{t}}=n_2(\mathbf{k}_\mathrm{t})\sin\theta_\mathrm{t}$ into Eqs. (S16b) and (S16c) yields

$$\phi=\arcsin\left(\frac{\overline{k}_{x_\mathrm{t}}}{n_1\sqrt{\beta^2\overline{k}_\mathrm{t}^2-2\beta\overline{k}_{z_\mathrm{t}}+1}}\right) \tag{S17a}$$

and

$$\psi=\arcsin\left(\frac{\beta\overline{k}_{x_\mathrm{t}}}{\sqrt{\beta^2\overline{k}_\mathrm{t}^2-2\beta\overline{k}_{z_\mathrm{t}}+1}}\right). \tag{S17b}$$

### B. Derivation of $\theta_{\mathrm{r}}(\mathbf{k}_{\mathrm{t}})$

Using time-reversal condition $\theta_{\mathrm{r}}(\beta, n_1) = \theta_{\mathrm{i}}(-\beta, n_1)$, we rewrite the critical reflection angle in terms of the critical transmission angle as

$$\theta_{\mathrm{r}} = \phi + \psi, \tag{S18}$$

where $\phi$ and $\psi$ are given in Eqs. (S16b) and (S16c) [or Eqs. (S17a) and (S17b)], respectively.

## IV. DERIVATION OF THE CRITICAL ANGLE EQUATIONS IN TABLE I

### A. Conveyor-Belt System [Fig. 1(b), Eqs. (2)]

#### 1. Frame-Hopping Method

In a stationary-interface – moving-matter system, such as the conveyor-belt system, the boundary conditions in the $K$ frame are simply

$$\omega_{\mathrm{i}} = \omega_{\mathrm{r}} = \omega_{\mathrm{t}} \tag{S19a}$$

and

$$k_{x_{\mathrm{i}}} = k_{x_{\mathrm{r}}} = k_{x_{\mathrm{t}}}. \tag{S19b}$$

Substituting these relations and the isotropic dispersion relation of medium 1, $k_{x_{\mathrm{i}}} = \frac{\omega_{\mathrm{i}} n_1}{c}\sin\theta_{\mathrm{i}}$, into the bianisotropic dispersion relation of medium 2 [Eq. (S7)], we get

$$\left(k_{z_{\mathrm{t}}} - \frac{\omega_{\mathrm{i}}}{c}\chi_2\right)^2 + \alpha_2\left(\frac{\omega_{\mathrm{i}} n_1}{c}\sin\theta_{\mathrm{i}}\right)^2 = \left(\alpha_2 n_2 \frac{\omega}{c}\right)^2, \tag{S20}$$

and obtain then the normal component of the transmission wavevector, $k_{z\mathrm{t}}$, as

$$k_{z_{\mathrm{t}}} = \frac{\omega_{\mathrm{i}}}{c}\left(\sqrt{\alpha_2^2 n_2^2 - \alpha_2 n_1^2 \sin^2\theta_{\mathrm{i}}} + \chi_2\right). \tag{S21}$$

We find the critical incidence angle, using the wave evanescence TIR criterion, by setting the radicand in Eq. (S21) to zero, which yields

$$\alpha_2^2 n_2^2 - \alpha_2 n_1^2 \sin^2\theta_{\mathrm{ic}} = 0, \tag{S22}$$

implying that

$$\theta_{\mathrm{ic}} = \arcsin\left(\sqrt{\alpha_2}\, n_2/n_1\right). \tag{S23}$$

Since the interface is stationary, we find the critical reflection angle as

$$\theta_{\mathrm{rc}} = \theta_{\mathrm{ic}} = \arcsin\left(\sqrt{\alpha_2}\, n_2/n_1\right). \tag{S24}$$

When $\theta_{\mathrm{i}} = \theta_{\mathrm{ic}}$, Eq. (S21) becomes

$$k_{z_{\mathrm{tc}}} = \frac{\omega_{\mathrm{i}}}{c}\chi_2, \tag{S25}$$

then substituting Eq. (S25) into Eq. (S7), gives

$$k_{x_{\mathrm{tc}}} = \frac{\omega_{\mathrm{i}}}{c}\sqrt{\alpha_2}\, n_2. \tag{S26}$$

Finally, substituting $k_{z_{\mathrm{tc}}}$ [Eq. (S25)] and $k_{x_{\mathrm{tc}}}$ [Eq. (S26)] into Eqs. (S10), we obtain the critical transmission phase and power angle as

$$\theta_{\mathrm{tc}}^{\mathbf{k}} = \arccos\left(\frac{\chi_2}{\sqrt{\alpha_2 n_2^2 + \chi_2^2}}\right) \tag{S27a}$$

and

$$\theta_{\mathrm{tc}}^{\mathbf{S}} = \pi/2, \tag{S27b}$$

respectively.

### 2. Catch-Up Method

Since the interface is stationary, we have, according to the catch-up limit ($v_{g_{zt}} = 0$), $\theta_{tc}^{\mathbf{S}} = \pi/2$, which yields $k_{z_{tc}} = \frac{\omega_i}{c}\chi_2$. Substituting this expression for $k_{z_{tc}}$ into Eq. (S7), we get $k_{x_{tc}} = \frac{\omega_i}{c}\sqrt{\alpha_2}n_2$, and find then $\theta_{tc}^{\mathbf{k}}$ as

$$\theta_{tc}^{\mathbf{k}} = \arccos\left(\frac{k_{z_{tc}}}{\sqrt{k_{z_{tc}}^2 + k_{x_{tc}}^2}}\right) = \arccos\left(\frac{\chi_2}{\sqrt{\alpha_2 n_2^2 + \chi_2^2}}\right). \tag{S28}$$

Using the phase-matching condition $\Delta k_x = 0$ at the interface gives

$$\sin\theta_{ic} = k_{x_{tc}}/k_1 = \sqrt{\alpha_2}n_2/n_1, \tag{S29}$$

which leads to

$$\theta_{ic} = \arcsin\left(\sqrt{\alpha_2}n_2/n_1\right) = \theta_{rc}. \tag{S30}$$

## B. Domino-Chain System [Fig. 1(c), Eqs. (c)]

In the interface frame, the $K'$ frame, which is co-moving with the moving interface, we have the frequency conservation condition $\Delta\omega' = 0$ and phase matching condition $\Delta k'_x = 0$. Applying the Lorentz transformation, we obtain then in the laboratory frame, the $K$ frame, the boundary conditions

$$\omega_i - \beta c k_{z_i} = \omega_r + \beta c k_{z_r} = \omega_t - \beta c k_{z_t} \tag{S31a}$$

and

$$k_{x_i} = k_{x_r} = k_{x_t}. \tag{S31b}$$

Moreover, with both media being isotropic, the dispersion relations are

$$k_x^2 + k_z^2 = (\omega n_1/c)^2 \tag{S32a}$$

and

$$k_x^2 + k_z^2 = (\omega n_2/c)^2, \tag{S32b}$$

respectively.

### 1. Frame-Hopping Method

Substituting $\omega_t = \omega_i - \beta c k_{z_i} + \beta c k_{z_t}$, $k_{z_i} = \frac{\omega_i n_1}{c}\cos\theta_i$ and $k_{x_t} = k_{x_i} = \frac{\omega_i n_1}{c}\sin\theta_i$ into Eq. (S32b), we obtain

$$k_{z_t} = \frac{\omega_i}{c}\frac{\beta n_2^2(1-\beta n_1\cos\theta_i) + \sqrt{n_2^2(1-\beta n_1\cos\theta_i)^2 - n_1^2\sin^2\theta_i(1-\beta^2 n_2^2)}}{1-\beta^2 n_2^2}. \tag{S33}$$

When the radicand in Eq. (S33) becomes negative, which occurs beyond the limit

$$n_2^2(1-\beta n_1\cos\theta_{ic})^2 - n_1^2\sin^2\theta_{ic}(1-\beta^2 n_2^2) = 0, \tag{S34}$$

the incident wave becomes totally reflected and TIR phenomenon occurs.

Solving Eq. (S34), we get

$$N = \frac{\sin\theta_{ic}}{\cos\theta_{ic} - \beta n_1} = -\frac{n_2}{\sqrt{n_1^2 - n_2^2}}, \tag{S35}$$

which leads to the angle-difference form [5]

$$\theta_{ic} = \arcsin\left(\frac{N\beta n_1}{\sqrt{1+N^2}}\right) - \arcsin\left(\frac{N}{\sqrt{1+N^2}}\right), \tag{S36}$$

where $\frac{N}{\sqrt{1+N^2}} = -n_2/n_1$.

After some algebraic manipulation, this formula simplifies to

$$\theta_{\rm ic} = \arcsin\left(n_2/n_1\right) - \arcsin\left(\beta n_2\right). \tag{S37}$$

Using the time-reversal condition $\theta_{\rm r}(\beta, n_1) = \theta_{\rm i}(-\beta, n_1)$, we get then the critical reflection angle

$$\theta_{\rm rc} = \arcsin\left(n_2/n_1\right) + \arcsin\left(\beta n_2\right). \tag{S38}$$

When $\theta_{\rm i} = \theta_{\rm ic}$, Eq. (S33) becomes

$$k_{z_{\rm t}} = \frac{\omega_{\rm i}}{c}\frac{\beta n_2^2(1-\beta n_1\cos\theta_{\rm i})}{1-\beta^2 n_2^2}. \tag{S39}$$

In Eq. (S39), $k_{z_{\rm tc}}$ is a function of the incidence frequency, $\omega_{\rm i}$. Substituting the boundary condition [Eq. (S31)] into Eq. (S39) leads to $k_{z_{\rm tc}}$ in terms of $\omega_{\rm t}$ as

$$k_{z_{\rm tc}} = \frac{\omega_{\rm t}}{c}\beta n_2^2. \tag{S40}$$

Finally, substituting Eq. (S40) into Eq. (S32b) yields the critical transmission angles

$$\theta_{\rm tc}^{\mathbf{k}} = \theta_{\rm tc}^{\mathbf{S}} = \arccos(\beta n_2). \tag{S41}$$

### *2. Catch-Up Method*

According to the catch-up limit, $v = v_2\cos\theta_{\rm t}^{\mathbf{S}}$, the critical transmission angles are $\theta_{\rm t}^{\mathbf{S}} = \theta_{\rm t}^{\mathbf{k}} = \arccos(\beta n_2) = \arcsin(\sqrt{1-\beta^2 n_2^2})$. To find the critical incidence and reflection angles, we use here the angle relation formulas in Sec. III, which are derived from the the boundary condition and the dispersion relations of the two media. This yields

$$\theta_{\rm ic} = \phi(\overline{k}_{\rm tc}) - \psi(\overline{k}_{\rm tc}) = \arcsin(n_2/n_1) - \arcsin(\beta n_2), \tag{S42}$$

and

$$\theta_{\rm rc} = \phi(\overline{k}_{\rm tc}) + \psi(\overline{k}_{\rm tc}) = \arcsin(n_2/n_1) + \arcsin(\beta n_2). \tag{S43}$$

## C. Moving-Truck System [Fig. 1(d), Eqs. (4)]

Since the interface also moves in the moving-truck system, we have the same boundary condition as in the domino-chain system in the laboratory frame, the $K$ frame [Eqs. (S31)]. Moreover, given that the two media are isotropic and bianisotropic, their dispersion relations are given in Eq. (S32a) and (S7), respectively.

### *1. Frame-Hopping Method*

Substituting $\omega_{\rm t} = \omega_{\rm i} - \beta c k_{z_{\rm i}} + \beta c k_{z_{\rm t}}$, $k_{z_{\rm i}} = \frac{\omega_{\rm i} n_1}{c}\cos\theta_{\rm i}$ and $k_{x_{\rm t}} = k_{x_{\rm i}} = \frac{\omega_{\rm i} n_1}{c}\sin\theta_{\rm i}$ into Eq. (S7), we obtain

$$k_{z_{\rm t}} = \gamma^2\frac{\omega_{\rm i}}{c}\left(\sqrt{n_2^2(1-\beta n_1\cos\theta_{\rm i})^2 - n_1^2\sin^2\theta_{\rm i}(1-\beta^2)} + \beta(1-\beta n_1\cos\theta_{\rm i})\right). \tag{S44}$$

When the radicand in Eq. (S44) becomes negative, which occurs beyond the limit

$$n_2^2(1-\beta n_1\cos\theta_{\rm ic})^2 - n_1^2\sin^2\theta_{\rm ic}(1-\beta^2) = 0, \tag{S45}$$

the incident wave becomes totally reflected and TIR phenomenon occurs.

Solving Eq. (S45), we get

$$N = \frac{\sin\theta_{\rm ic}}{\cos\theta_{\rm ic} - \beta n_1} = -\frac{n_2}{\sqrt{n_1^2 - \beta^2 n_1^2 - n_2^2 + \beta^2 n_1^2 n_2^2}}, \tag{S46}$$

which leads to the angle-difference form then we can find the critical incidence angle

$$\theta_{\mathrm{ic}} = \arcsin\left(\frac{N\beta n_1}{\sqrt{1+N^2}}\right) - \arcsin\left(\frac{N}{\sqrt{1+N^2}}\right), \tag{S47}$$

where $\frac{N}{\sqrt{1+N^2}} = -\frac{n_2}{n_1\sqrt{1-\beta^2+\beta^2 n_2^2}}$.

After some algebraic manipulations, this formula simplifies to

$$\theta_{\mathrm{ic}} = \arcsin\left(\frac{n_2}{n_1\sqrt{1-\beta^2+\beta^2 n_2^2}}\right) - \arcsin\left(\frac{\beta n_2}{\sqrt{1-\beta^2+\beta^2 n_2^2}}\right). \tag{S48}$$

Using time-reversal condition $\theta_{\mathrm{r}}(\beta, n_1) = \theta_{\mathrm{i}}(-\beta, n_1)$, we get then the critical reflection angle

$$\theta_{\mathrm{rc}} = \arcsin\left(\frac{n_2}{n_1\sqrt{1-\beta^2+\beta^2 n_2^2}}\right) + \arcsin\left(\frac{\beta n_2}{\sqrt{1-\beta^2+\beta^2 n_2^2}}\right). \tag{S49}$$

When $\theta_{\mathrm{i}} = \theta_{\mathrm{ic}}$, Eq. (S44) becomes

$$k_{z_{\mathrm{tc}}} = \gamma^2\beta\frac{\omega_{\mathrm{i}}}{c}(1-\beta n_1\cos\theta_{\mathrm{ic}}). \tag{S50}$$

In Eq. (S50), $k_{z_{\mathrm{tc}}}$ is a function of the incidence frequency, $\omega_{\mathrm{i}}$. Substituting the boundary condition [Eq. (S31a)] into Eq. (S50) leads to $k_{z_{\mathrm{tc}}}$ in terms of $\omega_{\mathrm{t}}$ as

$$k_{z_{\mathrm{tc}}} = \frac{\omega_{\mathrm{t}}}{c}\beta. \tag{S51}$$

Substituting Eq. (S51) into Eq. (S7) gives

$$k_{x_{\mathrm{tc}}} = \frac{\omega_{\mathrm{t}}}{c} n_2\sqrt{1-\beta^2}. \tag{S52}$$

Finally, substituting $k_{z_{\mathrm{tc}}}$ [Eq. (S51)] and $k_{x_{\mathrm{tc}}}$ [Eq. (S52)] into Eqs. (S10), we obtain the critical transmission phase and power angle as

$$\theta_{\mathrm{tc}}^{\mathbf{k}} = \arccos\left(\frac{\beta}{\sqrt{n_2^2+\beta^2-\beta^2 n_2^2}}\right) \tag{S53a}$$

and

$$\theta_{\mathrm{tc}}^{\mathbf{S}} = \arccos\left(\frac{\beta n_2}{\sqrt{1-\beta^2+\beta^2 n_2^2}}\right), \tag{S53b}$$

respectively.

### *2. Catch-Up Method*

Substituting the catch-up limit, $v = v_{\mathrm{g}}\cos\theta_{\mathrm{t}}^{\mathbf{S}}$, into Eq. (S9), we obtain

$$k_{z_{\mathrm{tc}}} = \frac{\omega_{\mathrm{t}}}{c}\beta \quad \text{and} \quad k_{x\mathrm{tc}} = \frac{\omega_{\mathrm{t}}}{c} n_2\sqrt{1-\beta^2}. \tag{S54a}$$

Substituting these expressions for $k_{z_{\mathrm{tc}}}$ and $k_{x_{\mathrm{tc}}}$ into Eqs. (S10), we find the critical transmission power angle and phase angle as

$$\theta_{\mathrm{tc}}^{\mathbf{S}} = \arccos\left(\frac{\beta n_2}{\sqrt{1-\beta^2+\beta^2 n_2^2}}\right) \tag{S54b}$$

and

$$\theta_{\rm tc}^{\mathbf{k}} = \arccos\left(\frac{\beta}{\sqrt{n_2^2+\beta^2-\beta^2 n_2^2}}\right), \tag{S54c}$$

respectively.

Applying angle relation formulas in Sec. III, we obtain the critical incidence angle and the critical reflection angle as

$$\theta_{\rm ic} = \phi(\overline{k}_{\rm tc}) - \psi(\overline{k}_{\rm tc}) = \arcsin\left(\frac{n_2}{n_1\sqrt{1-\beta^2+\beta^2 n_2^2}}\right) - \arcsin\left(\frac{\beta n_2}{\sqrt{1-\beta^2+\beta^2 n_2^2}}\right) \tag{S55}$$

and

$$\theta_{\rm rc} = \phi(\overline{k}_{\rm tc}) + \psi(\overline{k}_{\rm tc}) = \arcsin\left(\frac{n_2}{n_1\sqrt{1-\beta^2+\beta^2 n_2^2}}\right) + \arcsin\left(\frac{\beta n_2}{\sqrt{1-\beta^2+\beta^2 n_2^2}}\right), \tag{S56}$$

respectively.

## V. DERIVATION FOR THE MOST GENERAL MOVING INTERFACE – MOVING MATTER SYSTEM ($v \neq v_\mathrm{m}$)

### A. Catch-Up Criterion

Based on the catch-up limit, the transmitted wave becomes evanescent when $v = v_{\mathrm{g}z_\mathrm{t}}$. Then, in medium 2, we simplify Eq. (S9) into normalized form with the normalized wavevector $\overline{k}_{(z,x)_\mathrm{t}} = k_{(z,x)_\mathrm{t}}/(\omega_\mathrm{t}/c)$, and apply the catch-up limit, which yields

$$v = \beta c = v_{\mathrm{g}z_\mathrm{t}} = \frac{\overline{k}_{z_\mathrm{t}} - \chi_2}{\alpha_2^2 n_2^2 + \chi_2(\overline{k}_{z_\mathrm{t}} - \chi_2)} c, \tag{S57}$$

where $\alpha_2$ and $\chi_2$ are given in Eq. (S6c).

Solving Eq. (S57) for $\overline{k}_{z_\mathrm{tc}}$, we obtain

$$\overline{k}_{z_\mathrm{tc}} = \frac{\beta\alpha_2^2 n_2^2}{1 - \beta\chi_2} + \chi_2, \tag{S58a}$$

and substituting this expression into the dispersion relation of medium 2 [Eq. (S7)], we get the tangential wavevector $\overline{k}_{x_\mathrm{tc}}$ as

$$\overline{k}_{x_\mathrm{tc}} = \sqrt{\frac{\alpha_2^2 n_2^2 (1 - \beta\chi_2)^2 - (\beta\alpha_2^2 n_2^2)^2}{\alpha_2 (1 - \beta\chi_2)^2}}. \tag{S58b}$$

### B. Critical Transmission Group and Phase Angles

Substituting $\overline{k}_{z_\mathrm{tc}}$ [Eq.(S58a)] and $\overline{k}_{x_\mathrm{tc}}$ [Eq.(S58b)] into Eqs. (S10), we obtain the critical transmission group and phase angle as

$$\theta_\mathrm{tc}^\mathbf{S} = \arccos\left(\frac{\overline{k}_{z_\mathrm{tc}} - \chi_2}{\sqrt{\alpha_2^2 \overline{k}_{x_\mathrm{tc}}^2 + (\overline{k}_{z_\mathrm{tc}} - \chi_2)^2}}\right) = \arccos\left(\frac{\beta n_2}{\sqrt{(1-\beta\chi_2)^2/\alpha_2 + (1-\alpha_2)\beta^2 n_2^2}}\right) \tag{S59a}$$

and

$$\theta_\mathrm{tc}^\mathbf{k} = \arccos\left(\frac{\overline{k}_{z_\mathrm{tc}}}{\sqrt{\overline{k}_{x_\mathrm{tc}}^2 + \overline{k}_{z_\mathrm{tc}}^2}}\right) = \arccos\left(\frac{\beta(\alpha_2^2 n_2^2 - \chi_2^2) + \chi_2}{\sqrt{[\beta(\alpha_2^2 n_2^2 - \chi_2^2) + \chi_2]^2 + [\alpha_2^2 n_2^2 (1-\beta\chi_2)^2 - (\beta\alpha_2^2 n_2^2)^2]/\alpha_2}}\right), \tag{S59b}$$

respectively.

### C. Critical Incidence and Reflection Angles

Substituting $n_2(\mathbf{k}_\mathrm{t}) = \overline{k}_\mathrm{tc}$ and $\overline{k}_\mathrm{tc} = \sqrt{\overline{k}_{z_\mathrm{tc}}^2 + \overline{k}_{x_\mathrm{tc}}^2}$ into Eqs. (S17a) and (S17b) in Sec. III, we get the critical incidence angle and reflection angle as

$$\theta_\mathrm{ic} = \phi - \psi = \arcsin\left(\frac{\overline{k}_{x_\mathrm{tc}}}{n_1\sqrt{\beta^2 \overline{k}_\mathrm{tc}^2 - 2\beta\overline{k}_{x_\mathrm{tc}} + 1}}\right) - \arcsin\left(\frac{\beta\overline{k}_{x_\mathrm{tc}}}{\sqrt{\beta^2 \overline{k}_\mathrm{tc}^2 - 2\beta\overline{k}_{x_\mathrm{tc}} + 1}}\right) \tag{S60a}$$

and

$$\theta_\mathrm{rc} = \phi + \psi = \arcsin\left(\frac{\overline{k}_{x_\mathrm{tc}}}{n_1\sqrt{\beta^2 \overline{k}_\mathrm{tc}^2 - 2\beta\overline{k}_{x_\mathrm{tc}} + 1}}\right) + \arcsin\left(\frac{\beta\overline{k}_{x_\mathrm{tc}}}{\sqrt{\beta^2 \overline{k}_\mathrm{tc}^2 - 2\beta\overline{k}_{x_\mathrm{tc}} + 1}}\right), \tag{S60b}$$

where $\overline{k}_{z_\mathrm{tc}}$ and $\overline{k}_{x_\mathrm{tc}}$ are given in Eqs. (S59).

### 1. Stationary Interface – Moving Matter System: the Conveyor-Belt System

If $v = \beta c = 0$ and $v_{\rm m} = \beta_{\rm m} c \neq 0$, then $\overline{k}_{z_{\rm tc}}$ [Eqs. (S58a)] and $\overline{k}_{x_{\rm tc}}$ [Eqs. (S58b)] reduce to

$$\overline{k}_{z_{\rm tc}} = \chi_2 \tag{S61a}$$

and

$$\overline{k}_{x_{\rm tc}} = \sqrt{\alpha_2}\, n_2. \tag{S61b}$$

Substituting Eqs. (S61) into the critical angle formulas [Eqs. (S59) and (S60)], we obtain the same results in Table I [Eqs. (2)].

### 2. Moving Interface – Stationary Matter System: the Domino-Chain System

If $v_{\rm m} = \beta_{\rm m} c = 0$ and $v = \beta c \neq 0$, which means $\alpha_2 = 1$ and $\chi_2 = 0$, then $\overline{k}_{z_{\rm tc}}$ [Eqs. (S58a)] and $\overline{k}_{x_{\rm tc}}$ [Eqs. (S58b)] reduce to

$$\overline{k}_{z_{\rm tc}} = \beta n_2^2, \tag{S62a}$$

and

$$\overline{k}_{x_{\rm tc}} = n_2 \sqrt{1 - \beta^2 n_2^2}. \tag{S62b}$$

Substituting Eqs. (S62) into the critical angle formulas [Eqs. (S59) and (S60)], we obtain the same results in Table I [Eqs. (3)].

### 3. Moving Interface – Moving Matter System ($v = v_{\rm m}$): Moving-Truck System

If $v = v_{\rm m} = \beta c \neq 0$, then $\overline{k}_{z_{\rm tc}}$ [Eqs. (S58a)] and $\overline{k}_{x_{\rm tc}}$ [Eqs. (S58b)] reduce to

$$\overline{k}_{z_{\rm tc}} = \beta, \tag{S63a}$$

and

$$\overline{k}_{x_{\rm tc}} = n_2 \sqrt{1 - \beta^2}. \tag{S63b}$$

Substituting Eqs. (S63) into the critical angle formulas [Eqs. (S59) and (S60)], we obtain the same results in Table I [Eqs. (4)].

## VI. CATCH-UP GRAPHS FOR THE THREE SYSTEMS IN FIG. 1 (a)-(c)

Figure S1 shows the catch-up limit at a moving-perturbation interface for the domino-chain system, with medium 2 stationary, corresponding to a centered-circle isofrequency curve and $\mathbf{k}$ vector parallel to $\mathbf{S}$.

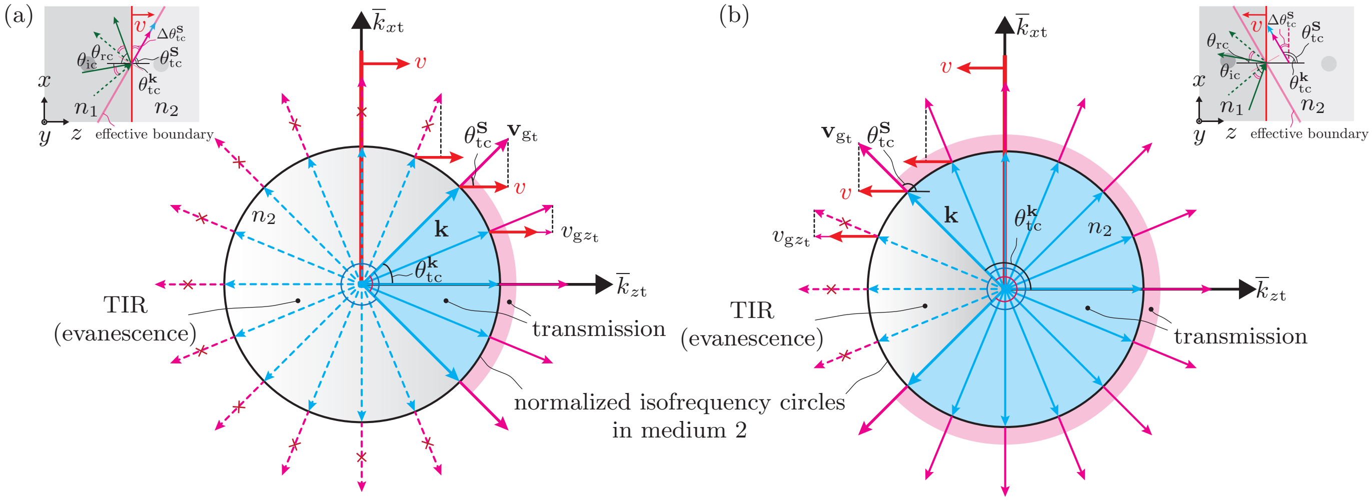


FIG. S1. Catch-up limit between the interface and the transmitted wave, shown here for the case of the domino-chain system. (a) $v > 0$. (b) $v < 0$. The blue, pink and gray regions correspond to the the sectors of phase transmission, power transmission and TIR (evanescence), respectively.

The catch-up graphs are simpler in the case of the conveyor-belt system and the static system, where the interface is stationary, i.e., $v = 0$ and $\theta_{\rm tc}^{\mathbf{S}} = \pi/2$. Figure S2 shows the catch-up limit of the conveyor-belt system, where the isofrequency curve of the bianistropic medium 2 is a left-shifted or right/shifted ellipse for molecules moving in the $+z$ or $-z$ directions, respectively, and $\mathbf{k}$ is not parallel to $\mathbf{S}$.

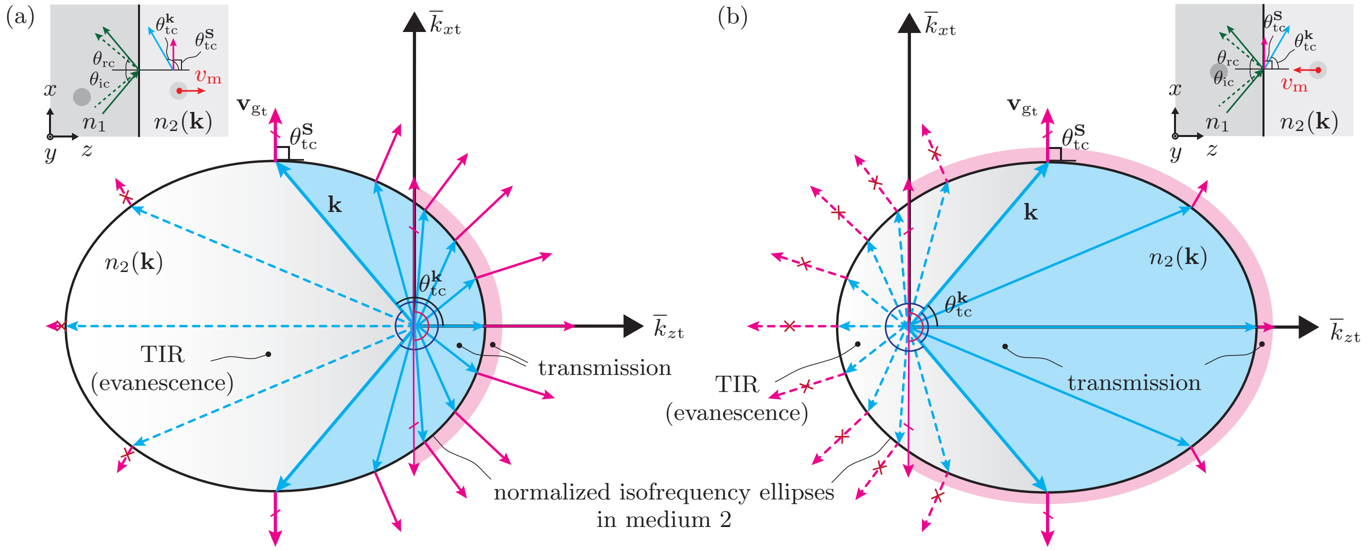


FIG. S2. Catch-up limit between the interface and the transmitted wave, shown here for the case of the conveyor-belt system. (a) $v_{\rm m} > 0$. (b) $v_{\rm m} < 0$. The blue, pink and gray regions correspond to the the sectors of phase transmission, power transmission and TIR (evanescence), respectively.

Figure S3 shows the catch-up limit at a conventional spatial interface corresponding to the static system.

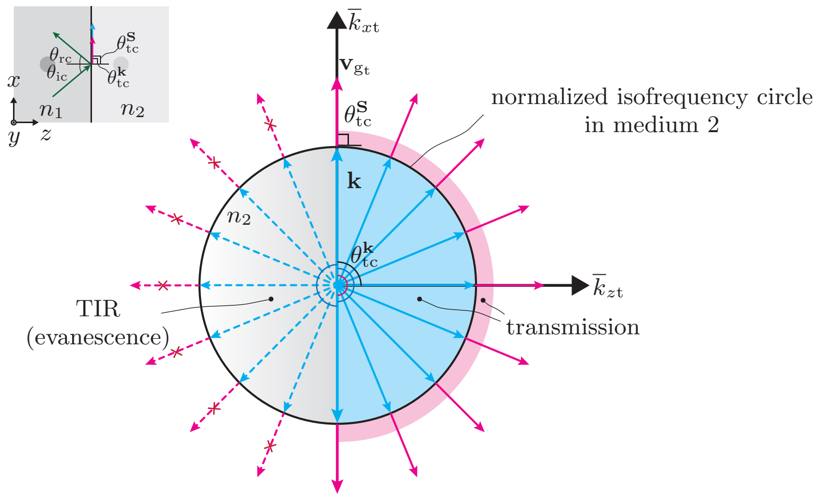


FIG. S3. Catch-up limit between the interface and the transmitted wave, shown here for the case of the static system. The blue, pink and gray regions correspond to the the sectors of phase transmission, power transmission and TIR (evanescence), respectively.

## VII. GENERALIZED SNELL'S LAW AND MOMENTUM DIAGRAM

### A. Snell's Law for Transmission

#### 1. General Case

Writing the dynamic boundary condition in terms of the effective refractive index leads to the generalized Snell's law of transmission

$$n_1 \sin\theta_\mathrm{i} = n_{2,\mathrm{eff}}(\theta_\mathrm{t}) \sin\theta_\mathrm{t}, \tag{S64a}$$

where

$$n_{2,\mathrm{eff}}(\theta_\mathrm{t}) = \frac{\omega_\mathrm{t}(\theta_\mathrm{t})}{\omega_\mathrm{i}} n_2(\theta_\mathrm{t}). \tag{S64b}$$

In the latter formula, the frequency-transformation part is given by

$$\frac{\omega_\mathrm{t}(\theta_\mathrm{t})}{\omega_\mathrm{i}} = \frac{1-\beta n_1 \cos\theta_\mathrm{i}}{1-\beta n_2(\theta_\mathrm{t})\cos\theta_\mathrm{t}}, \tag{S64c}$$

where

$$\cos\theta_\mathrm{i} = \frac{\beta n_2(\theta_\mathrm{t})^2 \sin\theta_\mathrm{t}^2 + (1-\beta n_2(\theta_\mathrm{t})\cos\theta_\mathrm{t})\sqrt{n_1^2(\beta^2 n_2(\theta_\mathrm{t})^2 - 2\beta n_2(\theta_\mathrm{t})\cos\theta_\mathrm{t} + 1) - n_2(\theta_\mathrm{t})^2 \sin\theta_\mathrm{t}^2}}{n_1(\beta^2 n_2(\theta_\mathrm{t})^2 - 2\beta n_2(\theta_\mathrm{t})\cos\theta_\mathrm{t} + 1)}, \tag{S64d}$$

while the motion-bianisotropy part is given by

$$n_2(\theta_\mathrm{t}) = \frac{\chi_2 \cos\theta_\mathrm{t} + \sqrt{\chi_2^2 \cos\theta_\mathrm{t}^2 - (\cos\theta_\mathrm{t}^2 + \alpha_2 \sin\theta_\mathrm{t}^2)(\chi_2^2 - \alpha_2^2 n_2^2)}}{\cos\theta_\mathrm{t}^2 + \alpha_2 \sin\theta_\mathrm{t}^2}. \tag{S64e}$$

#### 2. Particular Cases

In the domino-chain system, where only the interface moves, Eq. (S64b) reduces to

$$n_{2,\mathrm{eff}}(\theta_\mathrm{t}) = \frac{\omega_\mathrm{t}(\theta_\mathrm{t})}{\omega_\mathrm{i}} n_2, \tag{S65a}$$

and hence the frequency-transformation part reduces to

$$\frac{\omega_\mathrm{t}(\theta_\mathrm{t})}{\omega_\mathrm{i}} = \frac{1-\beta n_1 \cos\theta_\mathrm{i}}{1-\beta n_2 \cos\theta_\mathrm{t}}, \tag{S65b}$$

where

$$\cos\theta_\mathrm{i} = \frac{\beta n_2^2 \sin\theta_\mathrm{t}^2 + (1-\beta n_2 \cos\theta_\mathrm{t})\sqrt{n_1^2(\beta^2 n_2^2 - 2\beta n_2 \cos\theta_\mathrm{t} + 1) - n_2^2 \sin\theta_\mathrm{t}^2}}{n_1(\beta^2 n_2^2 - 2\beta n_2 \cos\theta_\mathrm{t} + 1)}. \tag{S65c}$$

In the conveyor-belt system, where only medium 2 moves, Eq. (S64b) reduces to

$$n_{2,\mathrm{eff}}(\theta_\mathrm{t}) = n_2(\theta_\mathrm{t}), \tag{S66}$$

with the motion-bianisotropy part Eq. (S64e).

In the static system where both the interface and the two media are stationary, Eq. (S64b) reduces to

$$n_{2,\mathrm{eff}}(\theta_\mathrm{t}) = n_2. \tag{S67}$$

## B. Snell's Law for Reflection

### 1. General Case

Similarly, writing the dynamic boundary condition in terms of the effective refractive index leads to the generalized Snell's law of reflection

$$n_1 \sin\theta_{\rm i} = n_{1,\rm eff}(\theta_{\rm r}) \sin\theta_{\rm r}, \tag{S68a}$$

where

$$n_{1,\rm eff}(\theta_{\rm r}) = \frac{\omega_{\rm r}(\theta_{\rm r})}{\omega_{\rm i}} n_1, \tag{S68b}$$

with the frequency-transformation part

$$\frac{\omega_{\rm r}(\theta_{\rm r})}{\omega_{\rm i}} = \frac{1-\beta n_1 \cos\theta_{\rm i}}{1+\beta n_1 \cos\theta_{\rm r}}, \tag{S68c}$$

where

$$\cos\theta_{\rm i} = \frac{(1+\beta^2 n_1^2)\cos\theta_{\rm r} 2 + \beta n_1}{\beta^2 n_1^2 + 2\beta n_1 \cos\theta_{\rm r} + 1}. \tag{S68d}$$

### 2. Particular Cases

In the domino-chain system, where the interface moves, since the first medium is always stationary, the formula for reflection is the same as Eq. (S68b).

In the conveyor-belt system and the static system, where the interface is stationary, Eq. (S64b) reduces to $n_{1,\rm eff}(\theta_{\rm t}) = n_1$.

## C. Momentum Diagram with Reflection

Figure S4 shows the momentum diagram for the reflected and transmitted waves in the three dynamic systems, using the generalized Snell's law given in Sec. VII A and VII B, where the transmission curves are the same as Fig. 3. In Fig. S4(a), the reflection curves are the same as the reflection curves in the domino-chain system because of the stationary interface. In Fig. S4(b) and (c), where the moving interface induces the frequency transformation of the reflected waves, the reflection momentum varies with the normal incidence wavevector, which also depends on the incidence angle. The reflection momentum curves are the same in the domino-chain system and moving-truck system when the interface velocity are the same.

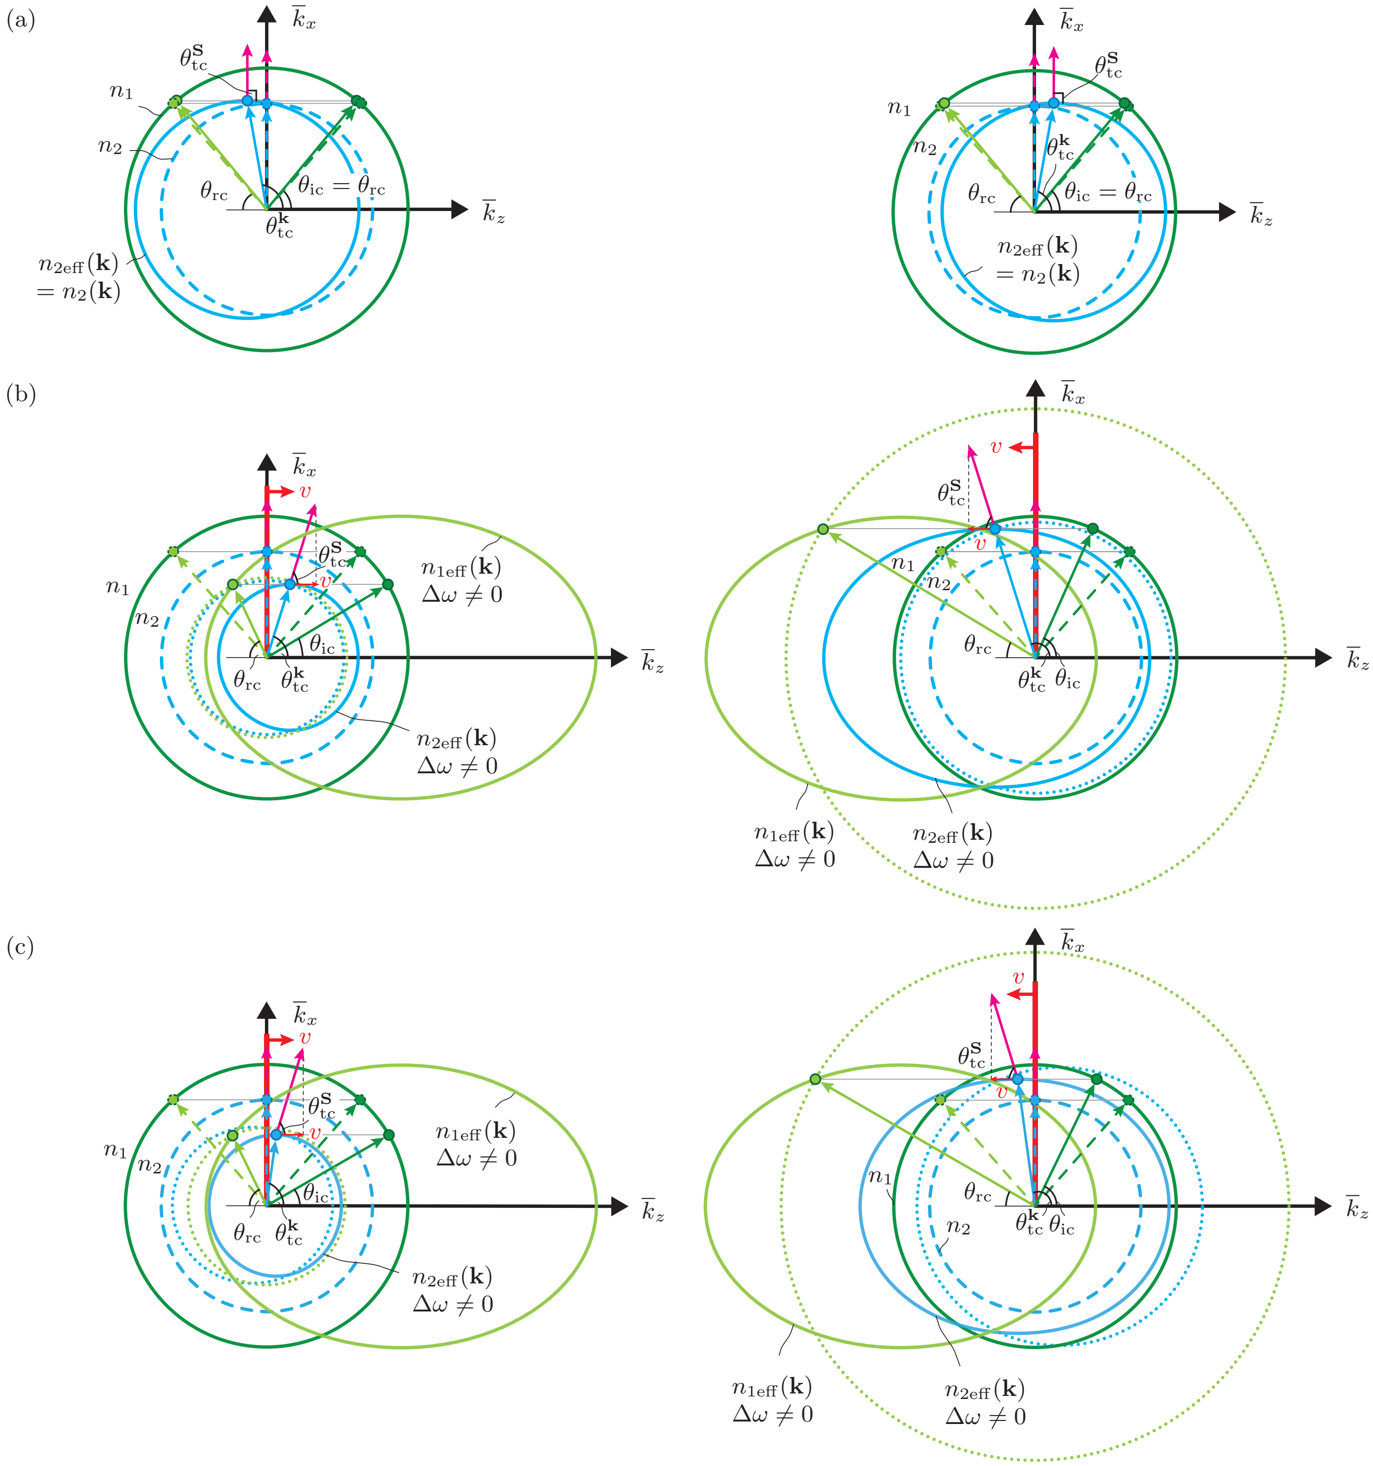


FIG. S4. Momentum diagrams for the incident, reflected and transmitted waves in terms of the normalized wavenumber $\bar{k}_{\rm i,r,t} = k_{\rm i,r,t}/(\omega_{\rm i}/c)$, along with critical angles, for the dynamic interfaces in Fig. 1, for $(n_1, n_2) = (2, 1.5)$ and both positive $z$-motion (left), with $\beta = 0.2$, and negative $z$-motion (right), with $\beta = -0.2$. (a) Conveyor-belt system. (b) Domino-chain system. (c) Moving-truck system. In all the cases, the dashed curves correspond to the static case. In the cases (b) and (c), the dotted blue curves are transmission isofrequency curves at $\theta_{\rm tc}^{\bf k}$ and the dotted green curves are reflection isofrequency curves at $\theta_{\rm rc}$.

## VIII. FULL-WAVE SIMULATION RESULTS

The data corresponding to the full-wave FDTD simulation results plotted in Fig. 4 are listed in Table SI and SII for the forward and backward case, respectively. The discrepancy of the simulation with respect to the (exact) theoretical values may come from the diffraction of the Gaussian incident beam, the tolerance in the selection of $\theta_{\mathrm{tc}}^{\mathbf{S}}$ and numerical errors. Nevertheless, the numerical results essentially follow the the mathematical formulas, and hence validate our theory. Additional numerical representations are shown in the supplemental animation file [6].

TABLE SI. Comparison of the theoretical and numerical results for the three dynamic systems in Fig. 1 with $\beta \geq 0$.

| Type | Angle | $\beta = 0$ | | | $\beta = 0.1$ | | | $\beta = 0.2$ | | | $\beta = 0.3$ | | | $\beta = 0.4$ | | |
|---|---|---|---|---|---|---|---|---|---|---|---|---|---|---|---|---|
| | | Theory/$\circ$ | FDTD/$\circ$ | Error/% | Theory/$\circ$ | FDTD/$\circ$ | Error/% | Theory/$\circ$ | FDTD/$\circ$ | Error/% | Theory/$\circ$ | FDTD/$\circ$ | Error/% | Theory/$\circ$ | FDTD/$\circ$ | Error/% |
| conveyor belt | $\theta_{\mathrm{ic}}$ | 48.59 | 50.17 | 3.25 | 49.00 | 51.64 | 5.39 | 50.38 | 52.70 | 4.61 | 53.24 | 54.90 | 3.12 | 59.23 | 62.42 | 5.39 |
| | $\theta_{\mathrm{rc}}$ | 48.59 | 50.17 | 3.25 | 49.00 | 51.64 | 5.39 | 50.38 | 52.70 | 4.61 | 53.24 | 54.90 | 3.12 | 59.23 | 62.42 | 5.39 |
| | $\theta_{\mathrm{tc}}^{\mathbf{k}}$ | 90.00 | 90.00 | 0.00 | 94.84 | 92.89 | 2.06 | 100.11 | 98.54 | 1.57 | 106.36 | 105.49 | 0.82 | 114.45 | 112.78 | 1.46 |
| | $\theta_{\mathrm{tc}}^{\mathbf{S}}$ | 90.00 | 90.00 | 0.00 | 90.00 | 88.06 | 2.16 | 90.00 | 88.47 | 1.70 | 90.00 | 89.18 | 0.91 | 90.00 | 88.47 | 1.70 |
| domino | $\theta_{\mathrm{ic}}$ | 48.59 | 49.98 | 2.86 | 39.96 | 40.03 | 0.18 | 31.13 | 31.67 | 1.73 | 21.85 | 20.78 | 4.90 | 11.72 | 11.12 | 5.12 |
| | $\theta_{\mathrm{rc}}$ | 48.59 | 49.98 | 2.86 | 57.22 | 55.70 | 2.66 | 66.05 | 67.00 | 1.44 | 75.33 | 72.51 | 3.74 | 85.46 | 82.44 | 3.53 |
| | $\theta_{\mathrm{tc}}^{\mathbf{k}}$ | 90.00 | 90.00 | 0.00 | 81.37 | 78.38 | 3.67 | 72.54 | 73.59 | 1.45 | 63.26 | 60.84 | 3.83 | 53.13 | 53.56 | 0.81 |
| | $\theta_{\mathrm{tc}}^{\mathbf{S}}$ | 90.00 | 90.00 | 0.00 | 81.37 | 78.38 | 3.67 | 72.54 | 73.59 | 1.45 | 63.26 | 60.84 | 3.83 | 53.13 | 53.56 | 0.81 |
| truck | $\theta_{\mathrm{ic}}$ | 48.59 | 50.60 | 4.14 | 39.62 | 39.86 | 0.61 | 30.02 | 28.51 | 5.03 | 20.07 | 19.91 | 0.80 | 10.00 | 10.43 | 4.30 |
| | $\theta_{\mathrm{rc}}$ | 48.59 | 50.60 | 4.14 | 56.76 | 55.40 | 2.40 | 64.07 | 61.31 | 4.31 | 70.58 | 70.13 | 0.64 | 76.42 | 78.78 | 3.09 |
| | $\theta_{\mathrm{tc}}^{\mathbf{k}}$ | 90.00 | 90.00 | 0.00 | 86.17 | 85.41 | 0.88 | 82.25 | 80.58 | 2.03 | 78.16 | 76.97 | 1.52 | 73.78 | 73.14 | 0.87 |
| | $\theta_{\mathrm{tc}}^{\mathbf{S}}$ | 90.00 | 90.00 | 0.00 | 81.43 | 80.68 | 0.92 | 72.97 | 71.42 | 2.12 | 64.75 | 63.73 | 1.58 | 56.79 | 56.31 | 0.85 |

TABLE SII. Comparison of the theoretical and numerical results for the three dynamic systems in Fig. 1 with $\beta \leq 0$.

| Type | Angle | $\beta = 0$ | | | $\beta = -0.1$ | | | $\beta = -0.2$ | | | $\beta = -0.3$ | | | $\beta = -0.4$ | | |
|---|---|---|---|---|---|---|---|---|---|---|---|---|---|---|---|---|
| | | Theory/$\circ$ | FDTD/$\circ$ | Error/% | Theory/$\circ$ | FDTD/$\circ$ | Error/% | Theory/$\circ$ | FDTD/$\circ$ | Error/% | Theory/$\circ$ | FDTD/$\circ$ | Error/% | Theory/$\circ$ | FDTD/$\circ$ | Error/% |
| conveyor belt | $\theta_{\mathrm{ic}}$ | 48.59 | 50.17 | 3.25 | 49.00 | 51.63 | 5.37 | 50.38 | 52.70 | 4.61 | 53.24 | 54.90 | 3.12 | 59.23 | 60.78 | 2.62 |
| | $\theta_{\mathrm{rc}}$ | 48.59 | 50.17 | 3.25 | 49.00 | 51.63 | 5.37 | 50.38 | 52.70 | 4.61 | 53.24 | 54.90 | 3.12 | 59.23 | 60.78 | 2.62 |
| | $\theta_{\mathrm{tc}}^{\mathbf{k}}$ | 90.00 | 90.00 | 0.00 | 85.16 | 87.11 | 2.29 | 79.89 | 81.46 | 1.97 | 73.64 | 74.51 | 1.18 | 65.55 | 63.24 | 3.52 |
| | $\theta_{\mathrm{tc}}^{\mathbf{S}}$ | 90.00 | 90.00 | 0.00 | 90.00 | 91.93 | 2.14 | 90.00 | 91.53 | 1.70 | 90.00 | 90.82 | 0.91 | 90.00 | 87.85 | 2.39 |
| domino | $\theta_{\mathrm{ic}}$ | 48.59 | 49.98 | 2.86 | 57.22 | 59.99 | 4.84 | 66.05 | 68.01 | 2.97 | 75.33 | 78.03 | 3.58 | 85.46 | 84.66 | 0.94 |
| | $\theta_{\mathrm{rc}}$ | 48.59 | 49.98 | 2.86 | 39.96 | 42.10 | 5.36 | 31.13 | 32.91 | 5.72 | 21.85 | 22.90 | 4.81 | 11.72 | 11.56 | 1.37 |
| | $\theta_{\mathrm{tc}}^{\mathbf{k}}$ | 90.00 | 90.00 | 0.00 | 98.63 | 98.96 | 0.33 | 107.46 | 110.20 | 2.55 | 116.74 | 117.00 | 0.22 | 126.87 | 122.89 | 3.14 |
| | $\theta_{\mathrm{tc}}^{\mathbf{S}}$ | 90.00 | 90.00 | 0.00 | 98.63 | 98.96 | 0.33 | 107.46 | 110.20 | 2.55 | 116.74 | 117.00 | 0.22 | 126.87 | 122.89 | 3.14 |
| truck | $\theta_{\mathrm{ic}}$ | 48.59 | 50.60 | 4.14 | 56.76 | 58.46 | 3.00 | 64.07 | 64.46 | 0.61 | 70.58 | 73.48 | 4.11 | 76.42 | 79.30 | 3.77 |
| | $\theta_{\mathrm{rc}}$ | 48.59 | 50.60 | 4.14 | 39.62 | 41.29 | 4.22 | 30.02 | 30.24 | 0.73 | 20.07 | 21.14 | 5.33 | 10.00 | 10.52 | 5.20 |
| | $\theta_{\mathrm{tc}}^{\mathbf{k}}$ | 90.00 | 90.00 | 0.00 | 93.83 | 95.88 | 2.18 | 97.75 | 98.75 | 1.02 | 101.84 | 102.16 | 0.31 | 106.22 | 105.14 | 1.02 |
| | $\theta_{\mathrm{tc}}^{\mathbf{S}}$ | 90.00 | 90.00 | 0.00 | 98.57 | 100.58 | 2.04 | 107.02 | 107.96 | 0.88 | 115.25 | 115.53 | 0.24 | 123.21 | 122.39 | 0.67 |

* lizhiyu@stu.xjtu.edu.cn


[1] Z.-L. Deck-Léger, N. Chamanara, M. Skorobogatiy, M. G. Silveirinha, and C. Caloz, Uniform-velocity spacetime crystals, Adv. Photonics **1**, 056002 (2019).

[2] E. J. Rothwell and M. J. Cloud, *Electromagnetics* (CRC press, 2018).

[3] Z.-L. Deck-Léger, X. Zheng, and C. Caloz, Electromagnetic wave scattering from a moving medium with stationary interface across the interluminal regime, Photonics **8**, 202 (2021).

[4] J. A. Kong, *Electromagnetic Wave Theory* (Wiley-Interscience, 1990).

[5] K. S. Kunz, Plane electromagnetic waves in moving media and reflections from moving interfaces, J. Appl. Phys. **51**, 873 (1980).

[6] See Supplemental Material at [URL will be inserted by publisher] for the FDTD illustration.
